# Supplementary material for: Physics-informed Neural Network Predictive Control for Quadruped Locomotion
Source: arXiv:2503.06995 source file (2025-03-10)
Supplement: Supplementary file 1 [file 7-appendix.tex]

The SuperArm model parameters are listed in table. I.

\begin{table}[h]
  \begin{center}
    \setlength{\abovecaptionskip}{-0.1 cm}
    \setlength{\belowcaptionskip}{-1 cm}
    \caption{Parameters of human and SuperLimb.}
    \label{tab:table1}
    \begin{tabular}{l|l|l} % <-- Alignments: 1st column left, 2nd middle and 3rd right, with vertical lines in between
      \textbf{Parameter} & \textbf{Value} & \textbf{Description}\\
      \hline
      $m_h$ & 0.001 $kg$ & The effective mass of \\
      & & human in the general model \\
      $I_h$ & 0.001 $kg \cdot m^2$ & The effective rotational \\
      & & inertia in the general model \\
      $m_1$ & 2.5 $kg$ & The mass of the 1st \\
      & & SuperLimb link \\
      $I_1$ & 0.01 $kg \cdot m^2$ & The rotational inertia of \\
      & & the 1st SuperLimb link \\
      $m_2$ & 1.2 $kg$ & The mass of the 2nd \\
      & & SuperLimb link \\
      $I_2$ & 0.01 $kg \cdot m^2$ & The rotational inertia of \\
      & & the 2nd SuperLimb link \\
      $m_3$ & 0.1 $kg$ & The mass of the 3rd \\
      & & SuperLimb link \\
      $I_3$ & 0.001 $kg \cdot m^2$ & The rotational inertia of \\
      & & the 3rd SuperLimb link \\
      $l_1$ & 0.2 $m$  & The length of 1st \\
      & & SuperLimb link \\
      $l_2$ & 0.2 $m$  & The length of 2nd \\
      & & SuperLimb link \\
      $l_3$ & 0.05 $m$  & The length of 3rd \\
      & & SuperLimb link \\
      $l_{11}$ & 0.05 $m$  & The position of 1st \\
      & & SuperLimb link CoM\\
      $l_{22}$ & 0.05 $m$  & The position of 2nd \\
      & & SuperLimb link CoM\\
      $l_{33}$ & 0.005 $m$  & The position of 3rd \\
      & & SuperLimb link CoM\\
    \end{tabular}
  \end{center}
\end{table}
